# Supplementary material for: Properties of Local Electronic Structures
Source: arXiv:2308.07780 ancillary file (2023-08-15)
Supplement: Supplementary file 1 [file si.pdf]

# Supporting Information: Properties of Local Electronic Structures

Frederik Ø. Kjeldal and Janus J. Eriksen*

*DTU Chemistry, Technical University of Denmark*

*Kemitorvet Bldg. 206, 2800 Kgs. Lyngby, Denmark*

E-mail: janus@dtu.dk

## 1 Theory

As noted in Sect. 2 of the main study, among the contributions to Eq. 1 associated with either the nuclear (nuc) or electronic (el) interactions between an atom $K$ and both its own local environment and its surroundings, the $E_K^{\text{nuc}}$ term is shared and defined as follows

$$E_K^{\text{nuc}} = \tfrac{1}{2}(\text{Tr}[\boldsymbol{V}_K\boldsymbol{D}] + Z_K \sum_{K \neq L}^{\mathcal{M}} \frac{Z_L}{|\boldsymbol{r}_K - \boldsymbol{r}_L|}) \ . \tag{S1}$$

In Eq. S1, $\boldsymbol{V}_K$ is the attractive potential associated with atom $K$, while $Z_K$ ($\boldsymbol{r}_K$) denote its charge (position), respectively. However, the corresponding $\bar{E}^{\text{el}}$ and $E_K^{\text{el}}$ terms to Eq. 1, as derived from the AO- and MO-based partitioning schemes, respectively, will generally differ. In the case of the latter, the electronic contribution reads

$$E_K^{\text{el}} = \text{Tr}[(\boldsymbol{T}_{\text{kin}} + \tfrac{1}{2}\boldsymbol{V}_{\text{nuc}})\boldsymbol{\delta}_K] + \tfrac{1}{2}\sum_{\sigma}\text{Tr}[\boldsymbol{G}_{\sigma}(\boldsymbol{D})\boldsymbol{\delta}_{K,\sigma}] + \text{Tr}[\boldsymbol{\epsilon}_{xc}(\boldsymbol{\rho})\boldsymbol{\varrho}_K] \ . \tag{S2}$$

The nuclear attraction and kinetic energy operators in Eq. S2 are denoted by $\boldsymbol{V}_{\text{nuc}}$ and $\boldsymbol{T}_{\text{kin}}$, respectively, alongside the effective Fock potential, $\boldsymbol{G}_{\sigma}$ ($\sigma = \alpha, \beta$ is a spin index), and the

energy density, $\boldsymbol{\epsilon}_{xc}$. In Eqs. S1 and S2, $\boldsymbol{D}$ denotes the spin-summed and orbital-invariant 1-electron reduced density matrix (1-RDM), while the objects that principally define this decomposition—the atom-specific 1-RDMs, $\{\boldsymbol{\delta}\}$—are constructed as follows:[S1]

$$\boldsymbol{\delta}_K = \sum_{\sigma} \boldsymbol{\delta}_{K,\sigma} = \sum_{\sigma} \sum_{i}^{\mathcal{N}_\sigma} \boldsymbol{d}_{i,\sigma} \boldsymbol{p}^K_{i,\sigma} \ . \tag{S3}$$

In turn, these are formulated via a set of 1-RDMs, $\boldsymbol{d}_{i,\sigma} = \boldsymbol{C}_{i,\sigma}\boldsymbol{C}^T_{i,\sigma}$, unique to the individual occupied spin-$\sigma$ MOs of the system, $\boldsymbol{C}_{i,\sigma}$, and a set of weights that distribute the 1-RDMs of all $\mathcal{N}_\sigma$ occupied MOs of $\alpha$-/$\beta$-spin on a given atom $K$, $\{\boldsymbol{p}^K\}$. Likewise, the total electronic density, $\boldsymbol{\rho}$, and its derivatives are all quantities that may be trivially defined in an atom-specific manner, $\{\boldsymbol{\varrho}\}$, by proceeding through the 1-RDMs, $\{\boldsymbol{\delta}\}$. Alternatively, as in the standard energy density analysis (EDA) scheme by Nakai,[S2,S3] one may instead partition $\boldsymbol{D}$ and $\boldsymbol{\rho}$ on account of which atoms individual AOs are localized on. This is done by limiting all trace operations in Eq. S2 to only those AOs that are spatially assigned to atom $K$

$$\bar{E}^{\text{el}}_K = \text{Tr}_{\mu\in K}[(\boldsymbol{T}_{\text{kin}} + \tfrac{1}{2}\boldsymbol{V}_{\text{nuc}})\boldsymbol{D}] + \tfrac{1}{2}\sum_{\sigma}\text{Tr}_{\mu\in K}[\boldsymbol{G}_\sigma(\boldsymbol{D})\boldsymbol{D}_\sigma] + \text{Tr}_{\mu\in K}[\boldsymbol{\epsilon}_{xc}(\boldsymbol{\rho})\boldsymbol{\rho}] \ . \tag{S4}$$

In the context of Eq. S4, it should be noted how a native EDA scheme may be extended through the use of either natural atomic orbitals or real-space grids,[S4,S5] both of which ameliorate the excessive basis-set dependence of the theory somewhat, but in standard (non-augmented) basis sets all such possible variants will yield comparable decompositions.

Included in both Eq. S1 and each of Eqs. S2 and S4 is a self-interaction contribution, given how $\boldsymbol{D} = \sum_K \boldsymbol{\delta}_K$ and $\boldsymbol{V}_{\text{nuc}} = \sum_K \boldsymbol{V}_K$. Thus, when using Eq. 1 to compute atomization energies, both $E^{\text{nuc}}_K$ and either of the two formulations in Eqs. S2 ($E^{\text{el}}_K$) and S4 ($\bar{E}^{\text{el}}_K$) effectively account for perturbations to nuclear-electronic interactions in moving from gas-phase to a molecular setting, with the frame of reference being ($i$) an atom and ($ii$) its associated electrons and the interactions with all other $\mathcal{M} - 1$ nuclei and their assigned electrons, re-

spectively. The nuclear term in Eq. S1 comprises a negative and a positive contribution, respectively, the sum of which denote the stabilization or destabilization of nucleus $K$ with respect to its resting state in vacuum. Likewise, both Eqs. S2 and S4 are made up of composite contributions of opposite signs, again of very similar absolute magnitude. In any of the two formulations, the first of these represents the stabilization of the electrons associated with atom $K$ from their attractive interactions with all surrounding nuclei, whereas the sum of the second and third terms gives the destabilization of an atom from the net increase in electron repulsion. The remaining part of Eqs. S2 and S4 gives the change in electronic kinetic energy of an atom upon embedding in a molecule and may be of either sign.

Finally, on par with Eq. 1, molecular dipole moments may be decomposed as

$$\boldsymbol{\mu} = \sum_{K}^{\mathcal{M}} \boldsymbol{\mu}_K^{\text{nuc}} + \boldsymbol{\mu}_K^{\text{el}} = \sum_{K}^{\mathcal{M}} \boldsymbol{\mu}_K^{\text{nuc}} + \bar{\boldsymbol{\mu}}_K^{\text{el}} \ . \tag{S5}$$

Again, the nuclear contributions are shared between the MO- and AO-based schemes

$$\boldsymbol{\mu}_K^{\text{nuc},\alpha} = Z_K \boldsymbol{r}_K^{\alpha} \ , \tag{S6}$$

while the corresponding electronic contributions again differ in the general case

$$\boldsymbol{\mu}_K^{\text{el},\alpha} = -\operatorname{Tr}[\tilde{\boldsymbol{\mu}}^{\alpha}\boldsymbol{\delta}_K] \tag{S7a}$$

$$\bar{\boldsymbol{\mu}}_K^{\text{el},\alpha} = -\operatorname{Tr}_{\mu\in K}[\tilde{\boldsymbol{\mu}}^{\alpha}\boldsymbol{D}] \ . \tag{S7b}$$

In Eqs. S6 and S7, the contributions are defined for each of the three Cartesian components $(\alpha = x, y, z)$ and expressed in terms of AO dipole integrals, $\tilde{\boldsymbol{\mu}}^{\alpha}$, in Eq. S7.

All decompositions of the present study were performed using the `decodense` package.[S6]

# 2 Additional Results

Table S1: IAO-based populations (in %) of IBOs from Figs. 3 and 4 of the main study.

| Bond | $w_a$ | $w_b$ | $\sum_i w_i$ |
|---|---|---|---|
| Acetaldehyde | | | |
| $C_1^a \cdots C_2^b$ | 50.1 | 49.8 | 99.9 |
| $C_2^a \cdots O^b$ | 38.6 | 61.2 | 99.8 |
| $C_2^a \cdots O^b$ | 35.3 | 64.0 | 99.3 |
| $C_2^a \cdots O^b$ | 3.0 | 93.2 | 96.2 |
| $C_2^a \cdots O^b$ | 0.1 | 99.7 | 99.8 |
| Acetone | | | |
| $C_1^a \cdots C_2^b$ | 50.2 | 49.5 | 99.7 |
| $C_2^a \cdots O^b$ | 38.9 | 60.9 | 99.8 |
| $C_2^a \cdots O^b$ | 33.4 | 65.1 | 98.5 |
| $C_2^a \cdots O^b$ | 3.1 | 93.7 | 96.8 |
| $C_2^a \cdots O^b$ | 0.1 | 99.6 | 99.7 |
| Acetic acid | | | |
| $C_1^a \cdots C_2^b$ | 48.9 | 50.4 | 99.3 |
| $C_2^a \cdots O_2^b$ | 39.4 | 60.5 | 99.9 |
| $C_2^a \cdots O_2^b$ | 30.4 | 68.6 | 99.0 |
| $C_2^a \cdots O_2^b$ | 5.5 | 91.4 | 96.9 |
| $C_2^a \cdots O_2^b$ | 0.2 | 99.6 | 99.8 |
| $C_2^a \cdots O_1^b$ | 35.3 | 64.3 | 99.6 |
| $C_2^a \cdots O_1^b$ | 7.8 | 90.2 | 98.0 |
| $C_2^a \cdots O_1^b$ | 0.6 | 99.0 | 99.6 |
| $O_1^a \cdots H_1^b$ | 68.5 | 30.9 | 99.4 |
| Dimethyl sulfoxide | | | |
| $C^a \cdots S^b$ | 50.4 | 49.3 | 99.7 |
| $S^a \cdots O^b$ | 99.0 | 0.0 | 99.0 |
| $S^a \cdots O^b$ | 40.4 | 59.1 | 99.5 |
| $S^a \cdots O^b$ | 5.1 | 90.0 | 95.1 |
| $S^a \cdots O^b$ | 2.4 | 94.6 | 97.0 |
| $S^a \cdots O^b$ | 0.0 | 99.9 | 99.9 |
| Dimethyl sulfone | | | |
| $C^a \cdots S^b$ | 49.4 | 50.2 | 99.6 |
| $S^a \cdots O^b$ | 37.6 | 61.4 | 99.0 |
| $S^a \cdots O^b$ | 7.0 | 89.7 | 96.7 |
| $S^a \cdots O^b$ | 4.6 | 91.0 | 95.6 |
| $S^a \cdots O^b$ | 0.3 | 99.3 | 99.6 |

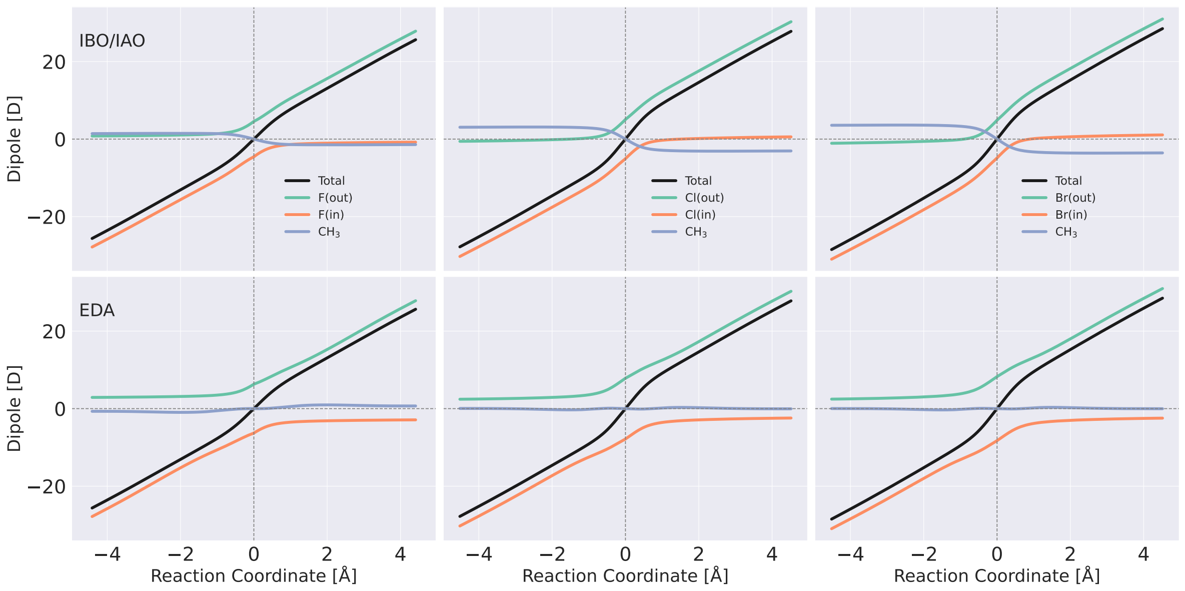


Figure S1: Same results as in Fig. 5 of the main study, but computed at the $\omega$B97M-V/pc-2 level of theory instead.

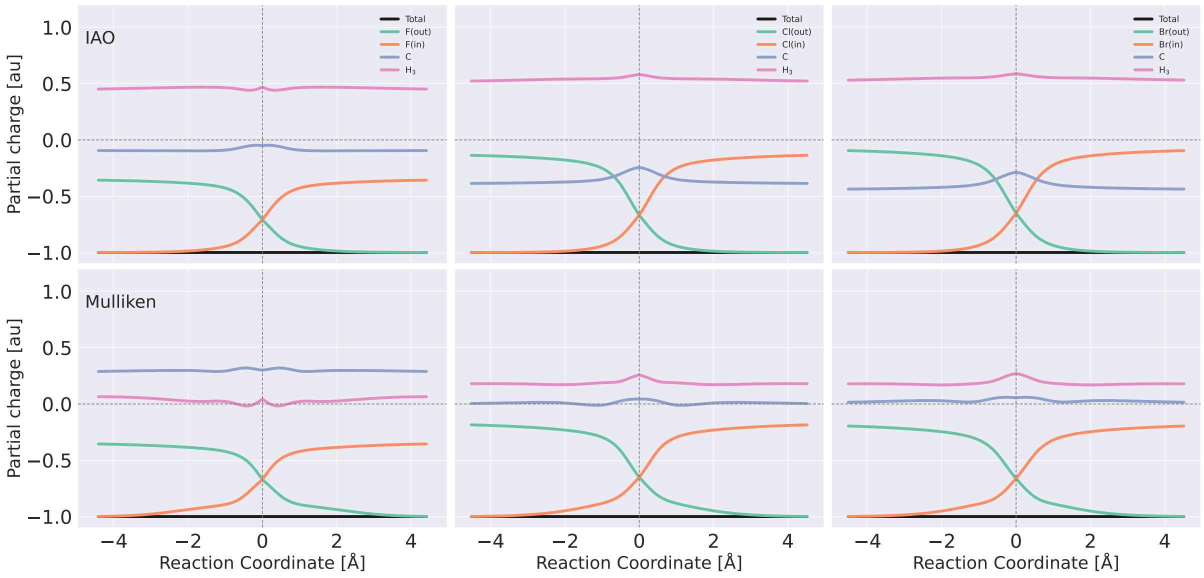


Figure S2: Same results as in Fig. 6 of the main study, but computed at the $\omega$B97M-V/pc-2 level of theory instead.

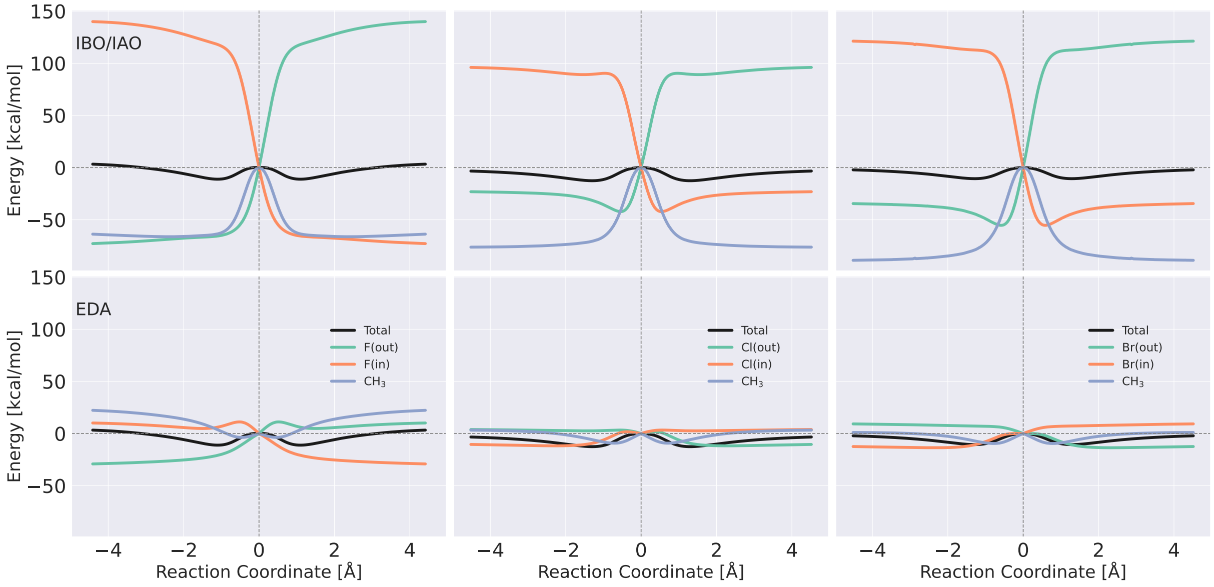


Figure S3: Same results as in Fig. 7 of the main study, but computed at the $\omega$B97M-V/pc-2 level of theory instead.

# References

(S1) Eriksen, J. J. Mean-Field Density Matrix Decompositions. J. Chem. Phys. **2020**, 153, 214109.

(S2) Nakai, H. Energy Density Analysis with Kohn-Sham Orbitals. Chem. Phys. Lett. **2002**, 363, 73.

(S3) Kikuchi, Y.; Imamura, Y.; Nakai, H. One-Body Energy Decomposition Schemes Revisited: Assessment of Mulliken-, Grid-, and Conventional Energy Density Analyses. Int. J. Quantum Chem. **2009**, 109, 2464.

(S4) Baba, T.; Takeuchi, M.; Nakai, H. Natural Atomic Orbital Based Energy Density Analysis: Implementation and Applications. Chem. Phys. Lett. **2006**, 424, 193.

(S5) Imamura, Y.; Takahashi, A.; Nakai, H. Grid-Based Energy Density Analysis: Implementation and Assessment. J. Chem. Phys. **2007**, 126, 034103.

(S6) Eriksen, J. J. `decodense`: A Decomposed Mean-Field Theory Code. `https://github.com/januseriksen/decodense`.
